# Supplementary material for: Optimal Stopping with Randomly Arriving Stopping Opportunities
Source: arXiv:2311.11098 source file (2026-08-29)
Supplement: Supplementary file 1 [file basis_functions.tex]

The crucial role of a proper choice of basis functions $\psi_l$ in \eqref{eq:basis} has been well established in the literature on Least Squares Monte Carlo. An important difference with typical applications of Least Squares Monte Carlo is that the basis functions for our problems also depend on time, $\psi_l(t,x,\theta)$, in contrast to $\psi_l(x,\theta)$, as one would have in a Bermudan option pricing problem.

Although optimized choices of basis functions may be derived for specific problems, we note two general principles that may guide the selection of basis functions.

First, note the dependence of $C(t,x,\theta)$ on time $t$ will typically be characterized mainly through the time to maturity, $T-t$. Indeed, the time to maturity governs on the one hand the window over which $Z$ may still move favorably and on the other hand the probability that we may not see another opportunity before maturity. It is therefore intuitive to use $T - t$ rather than $t$ as an argument to the basis functions.

Second, we can encode additional information about the continuation function by a judicious choice of basis functions. Suppose that $C_k(t', x', \theta') = c_k$ is known for all $k$ at some point $(t', x', \theta')$. By picking
\[\psi_0 \equiv 1 \text{ and }\psi_l(t', x', \theta') = 0,~ l > 1, \]
we have that $\widehat{C}_k(t', x', \theta') = \alpha_0$, so imposing $\alpha_0 = c_k$ in regression step $c_k$ ensures $\widehat{C}_k(t', x', \theta') = c_k$.

Similarly, suppose that we know that $\lim_{t \to T}C_k(t, x', \theta') = c_k$ at some point $(x', \theta')$. In this case, we may choose $(T, x', \theta')$ as the point in the previous paragraph along with continuous basis functions to ensure that $\lim_{t \to T}\widehat{C}_k(t, x', \theta') = c_k$. We use this in the choice of basis in Section \ref{sec:examples} to ensure that the estimated continuation value functions are continuous in $(t, x, \theta)$ at a special point of interest: the boundary point $(T,0)$ in Section \ref{sec:benchmark} and the boundary point $(T,\mathcal{K})$ in Section \ref{sec:maxcall}.
