# Supplementary material for: Optimal Stopping with Randomly Arriving Stopping Opportunities
Source: arXiv:2311.11098 source file (2026-08-29)
Supplement: Supplementary file 3 [file pseudo_pi.tex]

\todo[inline]{Do we really want a pseudo-algorithm besides what is in the main text? If so; I'll check whether this section is consistent with the current main text. }
Under Assumption~\ref{SA}, we suppose that we are given an input stopping family $\left(\sigma_{i}\right)$ satisfying \eqref{con}. Such a family may be obtained, for example, by the least squares method in Section~\ref{sec: fha and ls}, fixing some truncation level $K$ if necessary. That is, $\left(\sigma_{i}\right)$ may be given by
\begin{equation} \label{LSsig}
    \sigma_{i}:=\inf\left\{  j\geq i:Z(\tau_{j},X_{\tau_{j}})\geq\widehat{C}_{j}(\tau_{j},X_{\tau_{j}},\Theta_{\tau_{j}})\right\}\,.
\end{equation}
We then choose some window parameter $\kappa\geq1$ and improve this policy due to Proposition~\ref{polit}. We thus have to compute on a particular trajectory at time $\tau_{j}$ in $\left(X_{\tau_{j}},\Theta_{\tau_{j}}\right)$, $j \geq 0$,
\[ \mathbb{E}_{\mathcal{G}_{j}}\left[  U_{\sigma_{k}}\right] = \mathbb{E}_{\left(  \tau_{j},X_{\tau_{j}},\Theta_{\tau_{j}}\right)}\left[Z(\tau_{\sigma_{k}},X_{\tau_{\sigma_{k}}})\right],~j\leq k\leq j+\kappa\,, \]
which can be done by sub-simulations: Starting at $\tau_{j}^{(n)}$ in 
\[\left(X^{n,j},\Theta^{n,j}\right)\equiv\left(X_{\tau_{j}^{(n)}}^{(n)},\Theta_{\tau_{j}^{(n)}}^{(n)}\right)\]
on an outer trajectory with number $n$, $n=1,\ldots,N,$ simulate, for $m=1,\ldots,M$, sub-trajectories
\[ \left(X_{s}^{n,m,X^{n,j},\Theta^{n,j}},\Theta_{s}^{n,m,X^{n,j},\Theta^{n,j}}\right)_{s\geq\tau_{j}^{(n)}}\,, \]
and stopping times $\sigma_{k}^{n,m},$ $j\leq k\leq j+\kappa$, according to \eqref{LSsig}. Then construct
\[ \widehat{\sigma}_{0}^{(n)}:=\inf\left\{j \geq 0:Z(\tau_{j}^{(n)},X^{n,j})\geq\max_{j\leq k\leq j+\kappa}\frac{1}{M}\sum_{m=1}^{M}Z(\tau_{\sigma_{k}^{n,m}},X_{\tau_{\sigma_{k}^{n,m}}}^{n,m,X^{n,j},\Theta^{n,j}})\right\}\,, \]
and compute
\[ \frac{1}{N}\sum_{n=1}^{N}Z(\widehat{\sigma}_{0}^{(n)},X_{\widehat{\sigma}_{0}^{(n)}}^{(n)})\approx\mathbb{E}\left[  U_{\widehat{\sigma}_{0}}\right] = Y_{0}^{\widehat{\sigma}}\geq Y_{0}^{\sigma}\,. \]
