# Supplementary material for: Optimal Stopping with Randomly Arriving Stopping Opportunities
Source: arXiv:2311.11098 source file (2026-08-29)
Supplement: Supplementary file 4 [file pseudo_threshold.tex]

We now briefly outline how to create a reward-threshold based policy reminiscent of the methods outlined in \cite{A00}. The idea is to consider threshold strategies parametrized by $h_1,...,h_K$ as follows:
\begin{equation*}
\sigma_{k}=\inf\left\{k\leq j\leq K:~U_j\geq h_{j}\right\},~ k = 0,...,K
\end{equation*}
where we may set $h_K = 0$ without loss of generality, and we know that $\sigma_K = K$. It is clear that the optimal thresholds should satisfy the following recursive property:
\begin{align*}
h_{k} &:= \arg\max_{h\geq0}\mathbb{E}\left[U_k1_{\{U_k\geq h\}}+ U_{\sigma_{k+1}}1_{\{U_k<h\}}\right],~\\
\sigma_{k} &:= k1_{\{U_k\geq h_{k}\}}+\sigma_{k+1}1_{\{U_k<h_{k}\}}.
\end{align*}
For a straightforward Monte-Carlo approximation of this policy, we may sample trajectories $n=1,\ldots,N$, set $h_{K,N} = 0$ and $\sigma_{K,n} = K$, $n=1,\ldots,N$. Then, given $h_{k+1,N},\ldots,h_{K,N}$ and $\sigma_{k+1,n}\in\left\{k+1,\ldots,K\right\}$, $n=1,\ldots,N$, set
\begin{align*}
    h_{k,N} &:= \arg\max_{h\geq 0}\frac{1}{N}\sum_{n=1}^{N}\left(U_k^{(n)}1_{\{U_k^{(n)}\geq h\}}+Z_{\tau_{\sigma_{k+1,n}}}^{(n)}1_{\{U_k^{(n)}<h\}}\right)\,, \quad \text{and} \\
    \sigma_{k,n} &:= k1_{\{U_k^{(n)}\geq h_{k,N}\}}+\sigma_{k+1,n}1_{\{U_k^{(n)}<h_{k,N}\}}\,, \quad n=1,\ldots,N\,.
\end{align*}
