# Supplementary material for: Optimal Stopping with Randomly Arriving Stopping Opportunities
Source: arXiv:2311.11098 source file (2026-08-29)
Supplement: Supplementary file 5 [file appendix_pseudo.tex]

\begin{comment}
\subsection{Pseudoalgorithm PI}\label{app: pseudoalg PI}
\input{appendix_items/pseudo_pi}
\subsection{Pseudoalgorithm LSMC}\label{app:pseudoalg LS}
\input{appendix_items/pseudo_lsmc}

\subsection{Pseudoalgorithm threshold policy}\label{app:pseudoalg threshold}
\input{appendix_items/pseudo_threshold}
\end{comment}
